# Supplementary material for: Emphanitic anharmonicity in PbSe at high temperature and the anomalous electronic properties in the PbQ (Q=S, Se, Te) system
Source: arXiv:1805.01069 source file (2018-05-03)
Supplement: Supplementary file 1 [file SI-pbseEmphanisis.pdf]

# Supplementary Information: Emphanitic-like anharmonicity in PbSe at high temperature and the anomalous electronic properties in the PbQ (Q=S, Se, Te) system

Runze Yu,[1] Emil S. Bozin,[1,*] Milinda Abeykoon,[2] Boris Sangiorgio,[3] Nicola A. Spaldin,[3]
Christos D. Malliakas,[4] Mercouri G. Kanatzidis,[4,5] and Simon J. L. Billinge[1,6]

[1]*Condensed Matter Physics and Materials Science Department, Brookhaven National Laboratory, Upton, NY 11973, USA*
[2]*Photon Sciences Division, Brookhaven National Laboratory, Upton, NY 11973, USA*
[3]*Materials Theory, ETH Zurich, Wolfgang-Pauli-Strasse 27, CH-8093 Zurich, Switzerland*
[4]*Department of Chemistry, Northwestern University, Evanston, IL 60208, USA*
[5]*Materials Science Division, Argonne National Laboratory, Argonne, IL 60439, USA*
[6]*Department of Applied Physics and Applied Mathematics, Columbia University, New York, NY 10027, USA*

## MODELING LOCAL PB OFF-CENTERING IN PBSE

To explore whether the experimental PDF data of PbSe are consistent with there being local Pb off-centering the approach that was previously taken in [1] was used. Structural models were refined over the range 2.6 Å to 5.7 Å (the low-$r$ region of the PDF that yields local structural information) using the program PDFgui [2]. Four different models were compared to each other by refining to the PDF data at each temperature. The details of the model are described in [1] and summarized here:

1. The conventional crystallographic cubic rock-salt (Fm-3m), labeled 000 relaxed in Figure 3 in the main paper. This model has 3 refinable parameters: lattice parameter and ADPs of Pb and Se.

2. "000" model. In this model the same rock-salt model as above was refined using one parameter (lattice parameter) only but with the ADP parameters of Pb and Se constrained to the values predicted at each temperature from the Debye model without any offset.

3. 100 model. This is a distorted model with a tetragonal unit cell, but with no displacements of Pb allowed off special positions within the unit cell. This model has 2 parameters, $a$ and $b$. The ADPs values are fixed in the same way as the 000 model.

4. 100 PbO-like, displacements of Pb are allowed along the unique axis in the tetragonal cell, with a displacement pattern resembling that in PbO [3]. This model has 3 refinable parameters, $a$, $b$ and $\delta$, the Pb displacement amplitude. The ADP values are constrained in the same way as in the 000 model.

## DEBYE MODEL AND THE DETERMINATION OF THE $\Delta U_{iso}$ FOR THE ADP OF PB IN PBSE

The canonical temperature dependence of the ADPs, $U_{iso}$, was modelled using the Debye Model [4],

$$U_{iso}(T) = \frac{3h^2}{2\pi^2 m k_B \theta_D}\left(\frac{\phi\left(\frac{\theta_D}{T}\right)}{\frac{\theta_D}{T}} + \frac{1}{4}\right) + U_{off}, \tag{1}$$

where $h$ is the Planck constant, $m$ is the atomic mass, $k_B$ is the Boltzmann constant, $\theta_D$ is the Debye temperature and

$$\phi(x) = \frac{1}{x}\int_0^x \frac{x' dx'}{\exp(x') - 1}. \tag{2}$$

$U_{off}$ describes any static disorder in the system which explains a value of $U_{iso}(T = 0)$ that is larger than expected from the quantum zero-point motion. In this Debye model, there are only two refinable parameters: Debye temperature $\theta_D$, and $U_{off}$.

Any deviation from Debye behavior is typically ascribed either to the presence of significant anharmonicity or inadequacy of the structural model used in the form of the presence of nanoscale structural distortions that do not propagate over long lengthscales [1] and are therefore unaccounted for by the average structural model.

The first step is to extract $U_{iso}(T)$ values from the PbSe xPDF data at each temperature by refining the rock-salt model to the PDF data at each temperature. The ADPs were extracted by fitting over the range $10 < r < 50$ Å using PDFgui [2]. The Debye model was then fit to the Pb ADPs over the temperature range from 10-150 K. The expected (in the harmonic approximation) ADPs are then given by the values obtained by extrapolating this Debye curve to higher temperatures (blue line in Figure S1). The actual measured ADPs of lead deviate upwards from this curve starting at around $T = 150$ $K$. The measured ADPs are rather well fit in the high-$T$ region by taking the same Debye curve (fixed $\theta_D$) but offsetting it upwards by an amount $\Delta U_{off}$, where $\Delta U_{off}$ is obtained by fixing the parameters from the blue Debye curve and refining an additional

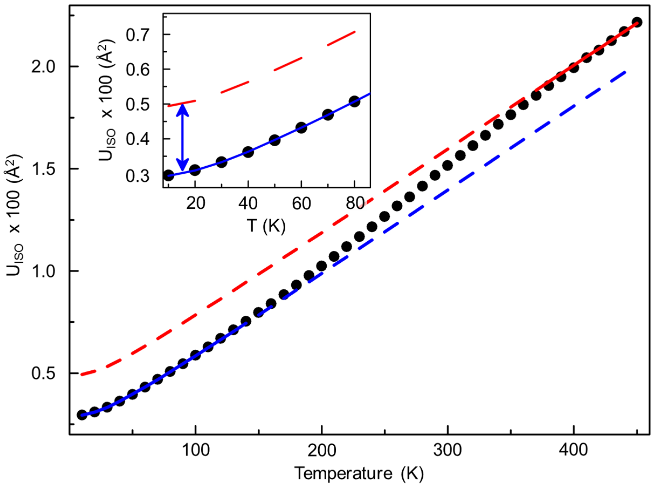


FIG. S1. Debye model fitting the Pb ADPs in PbSe extracted from the xPDF data with the fitting range from 2-30 Å. The Pb ADPs extracted from fitting are shown as the black symbols. The blue and red lines show the fitting curve to the low temperature and high temperature data, respectively. The lines are shown as solid over the range that they were fit, and where they are dashed they are extrapolated using the parameters from the fit region. The inset shows the low-temperature region on an expanded scale.

offset, $\Delta U_{off}$, so that the Debye curve goes through the high-$T$ data in the range $375 \leq T \leq 480$ K. This results in a new Debye curve shown in Red in Fig. S1.

## FIRST-PRINCIPLES COMPUTATIONS

Our first-principles calculations were performed using the PAW [5, 6] implementation of density functional theory (DFT) as in the VASP package [7]. Spin-orbit coupling was included and we used a plane-wave energy cutoff of 600 eV. For PbQ we used the PBEsol [8] exchange-correlation functional, the equilibrium volume as obtained after a full structural relaxation, and a $20 \times 20 \times 20$ $\Gamma$-centered $k$-point mesh. For NaCl we used the LDA exchange-correlation functional [9], the equilibrium volume as obtained after a full structural relaxation, and a $15 \times 15 \times 15$ $\Gamma$-centered $k$-point mesh. For $PbTiO_3$ we used the LDA exchange-correlation functional, the theoretical tetragonal structure [10], and a $15 \times 15 \times 13$ $\Gamma$-centered $k$-point mesh. For $BaTiO_3$ we used the LDA exchange-correlation functional, the theoretical tetragonal structure [11], and a $15 \times 15 \times 14$ $\Gamma$-centered $k$-point mesh. For $LaAlO_3$ we used the PBEsol exchange-correlation functional, the experimental cubic structure [12], and a $15 \times 15 \times 15$ $\Gamma$-centered $k$-point mesh.

The structural distortion was modeled as a global ferroelectric distortion. While this situation of course differs from the actual correlated local dipole behavior at the heart of the emphanisis, we expect the extracted

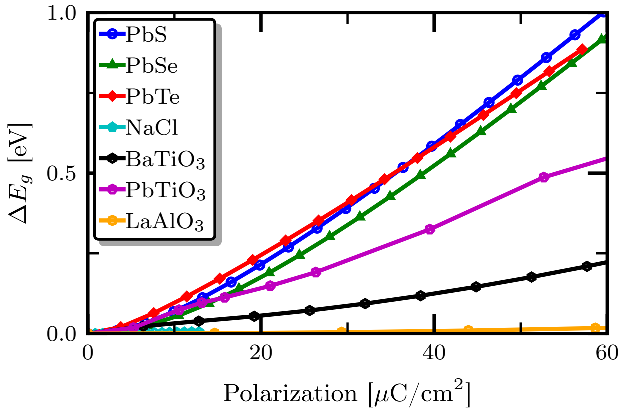


FIG. S2. Change in band gap for the studied compounds as a function of the polarization resulting from the ferroelectric distortion. The polarization was computed taking into account the Born effective charges from Refs. [11, 13]; for NaCl and $LaAlO_3$ we used the nominal charges.

trends between materials to be similar. For the rocksalt systems the distortion was modeled by a displacement of the cations along the [100] direction, while for the perovskite structures we used the ferroelectric distortion in the tetragonal phase (for $LaAlO_3$ we used the displacement pattern of $PbTiO_3$). Figure S2 shows the obtained evolution of the band gap as a function of the polarization (computed using the Born effective charges from Refs. [11, 13]) resulting from the distortion. In all compounds one can see an increase of the band gap with increasing distortion (polarization). For the systems without any tendency for a ferroelectric distortions (NaCl and $LaAlO_3$) the band gap almost does not change, for a ferroelectric compound as $BaTiO_3$ the effects start to be appreciable, and are largest for the compounds with a lone pair ($PbTiO_3$ and PbQ). Interestingly, the PbQ systems show the most pronounced effects, and within this class PbSe the smallest effect. While this may be a coincidence in our calculations, it is also consistent with the total scattering experiments presented in the main text. There we found the smallest emphanitic response in PbSe.

* bozin@bnl.gov

[1] E. S. Božin, C. D. Malliakas, P. Souvatzis, T. Proffen, N. A. Spaldin, M. G. Kanatzidis, and S. J. L. Billinge, Science **330**, 1660 (2010), URL `http://www.sciencemag.org/content/330/6011/1660`.

[2] C. L. Farrow, P. Juhás, J. Liu, D. Bryndin, E. S. Božin, J. Bloch, T. Proffen, and S. J. L. Billinge, J. Phys: Condens. Mat. **19**, 335219 (2007), URL `http://iopscience.iop.org/0953-8984/19/33/335219/`.

[3] P. Boher, P. Garnier, J. Gavarri, and A. Hewat, J. Solid State Chem. **57**, 343 (1985).

[4] P. Debye, Ann. Phys.-Berlin **39**, 789 (1912).

[5] P. E. Blöchl, Phys. Rev. B **50**, 17953 (1994).

[6] G. Kresse and D. Joubert, Phys. Rev. B **59**, 1758 (1999).

[7] G. Kresse and J. Furthmüller, Phys. Rev. B **54**, 11169 (1996).

[8] J. P. Perdew, A. Ruzsinszky, G. I. Csonka, O. A. Vydrov, G. E. Scuseria, L. A. Constantin, X. Zhou, and K. Burke, Phys. Rev. Lett. **100**, 136406 (2008), URL `https://link.aps.org/doi/10.1103/PhysRevLett.100.136406`.

[9] J. P. Perdew and A. Zunger, Phys. Rev. B **23**, 5048 (1981).

[10] A. García and D. Vanderbilt, Phys. Rev. B **54**, 3817 (1996).

[11] P. Ghosez, *First-principles study of the dielectric and dynamical properties of barium titanate*.

[12] A. Nakatsuka, O. Ohtaka, H. Arima, N. Nakayama, and T. Mizota, Acta Cryst. E **61**, i148 (2005).

[13] U. Waghmare, N. A. Spaldin, H. Kandpal, and R. Seshadri, Phys. Rev. B **67**, 125111 (2003).
